# Supplementary material for: Measurement of the $C\!P$ violation parameter $A_\Gamma$ in $D^0 \to K^+K^-$ and $D^0 \to \pi^+\pi^-$ decays
Source: arXiv:1702.06490 source file (2017-08-07)
Supplement: Supplementary file 1 [file supplementary-app.tex]

\clearpage

\section*{Supplementary material for LHCb-PAPER-2016-063}
\label{sec:Supplementary-App}

Figures~\ref{fig:D0_mass_window}, \ref{fig:pseudoAG-raw_SM}, \ref{fig:results_dtokk}, \ref{fig:results_dtopipi} and \ref{fig:secondaries_SM} 
are from the analysis based on Eq.~\eqref{eq:Aind} 
and Figs.~\ref{fig:unbinned:mass_KK}, \ref{fig:unbinned:mass_PiPi}, \ref{fig:unbinned:time_KK}, \ref{fig:unbinned:time_PiPi},
\ref{fig:unbinned:asym_KK} and \ref{fig:unbinned:asym_PiPi} from the analysis based on Eq.~\eqref{eq:A_G}.

\begin{figure}[tbh]
\centering
\includegraphics[width=0.5\textwidth]{Fig5a} 
\includegraphics[width=0.48\textwidth]{Fig5b} 
\caption{Distribution of the invariant mass difference $\Delta m \equiv m(\Dz\pip) - m(\Dz)$,
 in the 2012 \MagDown subsample for  the (left) \decay{\Dz}{\Kp \Km}  
and  (right) \decay{\Dz}{\pip \pim} candidates,  with results of the fits included. Black dots are data points, while the solid blue line is 
the total fit projection. The signal component is represented by the dashed green line, 
while the random pion background is represented by the filled purple
area. Dashed red and dash-dotted purple lines indicate signal and sideband regions respectively. 
A Johnson $S_U$-distribution
plus the sum of three Gaussian functions is used to model the signal, while 
the background is described by an empirical function of the form $1 - \exp [(\Delta m - \Delta m_0)/\alpha] + \beta(\Delta m/\Delta m_0 - 1)$, 
where $\Delta m_0$ is the threshold of the function, and $\alpha$ and $\beta$ describe its shape.
The residuals between data and the fit are shown in units of the statistical standard deviation, labelled as pull.
}
\label{fig:D0_mass_window}
\end{figure}
 %%%%%%%%%%%%%%%%%%%%%%%%%%%%%%%%%%%%%%%%%%%%%%%%%%%%%%%%%%%%%%%%%%%%%

%
\begin{figure}[tbh]
\centering 
\includegraphics[width=0.4944\textwidth]{Fig6a} 
\includegraphics[width=0.4944\textwidth]{Fig6b} \\
\includegraphics[width=0.4944\textwidth]{Fig6c}  
\includegraphics[width=0.4944\textwidth]{Fig6d} 
\caption{Measured (top left) raw asymmetry and (bottom left) corrected  asymmetry  in bins of $t/\tau_D$, where $\tau_D = 0.410\ps$~\cite{PDG2016},  
for the \decay{\Dz}{\Km\pip} decay mode.  
The results obtained in the four subsamples are shown, with fit results included (dashed lines). 
Results for $\agamma(\decay{\Dz}{\Km\pip})$ (top)~before and (bottom) after the correction are reported on the right, 
where the label  2011 (2012) is abbreviated 11 (12) and \MagUp (\MagDown) is abbreviated $\mathrm{U}(\mathrm{D})$.
The weighted average (avg.) of the four \agamma values is indicated by the colored vertical band.}
\label{fig:pseudoAG-raw_SM}
\end{figure}
%%%%%%%%%%%%%%%%

\begin{figure}[tbh]
\centering
\includegraphics[width=0.4944\textwidth]{Fig7a} 
\includegraphics[width=0.4944\textwidth]{Fig7b} \\
\includegraphics[width=0.4944\textwidth]{Fig7c}  
\includegraphics[width=0.4944\textwidth]{Fig7d} 
\caption{Measured (top left) raw asymmetry and (bottom left) corrected  asymmetry  in bins of $t/\tau_D$, where $\tau_D = 0.410\ps$~\cite{PDG2016},  
for the \decay{\Dz}{\Kp\Km} decay mode.
The results obtained in the four subsamples are shown, with fit results included (dashed lines). 
Results for $\agamma(\decay{\Dz}{\Kp\Km})$  (top) before and
(bottom) after  the correction are reported on the right, 
where the label  2011 (2012) is abbreviated 11 (12) and \MagUp (\MagDown) is abbreviated $\mathrm{U}(\mathrm{D})$.
The weighted average (avg.) of the four \agamma values is indicated by the colored vertical band.}
\label{fig:results_dtokk}
\end{figure}

%%%%%%%%%%%%%%%%%
\begin{figure}[tbh]
\centering
\includegraphics[width=0.4944\textwidth]{Fig8a} 
\includegraphics[width=0.4944\textwidth]{Fig8b} \\
\includegraphics[width=0.4944\textwidth]{Fig8c}  
\includegraphics[width=0.4944\textwidth]{Fig8d} 
\caption{Measured (top left) raw asymmetry and (bottom left) corrected  asymmetry  in bins of $t/\tau_D$, where $\tau_D = 0.410\ps$~\cite{PDG2016},  
for the  \decay{\Dz}{\pip\pim} decay mode.
The results obtained in the four subsamples are shown, with fit results included (dashed lines). 
Results for $\agamma(\decay{\Dz}{\pip\pim})$  (top) before  and
(bottom)  after the correction are reported on the right, 
where the label  2011 (2012) is abbreviated 11 (12) and \MagUp (\MagDown) is abbreviated $\mathrm{U}(\mathrm{D})$.
The weighted average (avg.) of the four \agamma values is indicated by the colored vertical band.}
\label{fig:results_dtopipi}
\end{figure}
%%%%

\begin{figure}[tbh]
\centering
\includegraphics[width=0.46\textwidth]{Fig9a} 
\includegraphics[width=0.49\textwidth]{Fig9b} 
\caption{Distribution (left) of $\ln(\chisqip(\Dz))$ with $t/\tau_D
\in [5.55, 20]$ in the 2012 \MagDown subsample,  with fit results
overlaid, and (right)  fraction of secondary decays \fsec as a function of $t/\tau_D$.
These plots illustrate the method used to estimate the relative fraction of secondary charm decays \fsec.
For large decay times $(t/\tau_D>3.4)$, where the secondary component
is sizable and well distinguishable from the prompt component,
a fit of the distribution of $\chisqip(\Dz)$  in each bin allows the estimation of \fsec from data, 
both with and without the $\chisqip(\Dz)<9$ requirement. An example of these fits is reported on the left, 
corresponding to the higher time bin. The values of \fsec without $\chisqip(\Dz)$ requirement are used to constrain the normalization 
of an acceptance-corrected analytical model of the number of secondary decays, 
given by the convolution of two exponentials having as slopes the average lifetime
of a mixture of $b$~hadrons ($\tau_b = 1.568\ps$~\cite{PDG2016})  and  the average lifetime of the \Dz\ meson 
($\tau_D = 0.410\ps$~\cite{PDG2016}).  The value of \fsec in the final sample with all requirements is then obtained
by interpolation of the low-decay-time part of the model, that is
unaffected by requirements, and the points at large decay times measured from data as explained above.  
}
\label{fig:secondaries_SM}
\end{figure}

%%%%%%%%%%%%%%%%%%%%%%%%%%%%%%%%%%%%%
%%%%%%%%%%%%%%%%%%%%%%%%%%%%%%%%%%%%%
%%% %%%%Swimming-based analysis
%%%%%%%%%%%%%%%%%%%%%%%%%%%%%%%%%%%%%
%%%%%%%%%%%%%%%%%%%%%%%%%%%%%%%%%%%%%
\begin{figure}[tbh]
\centering
\includegraphics[width=0.49\textwidth]{Fig10a} 
\includegraphics[width=0.49\textwidth]{Fig10b} 
\caption{Distributions of (left) $m(\Kp\Km)$ and (right) $\Delta m$ for the 
the selected \decay{\Dstar}{\Dz}{\pip}, \decay{\Dz}{\Kp\Km} candidates 
in the second of the three 2012 data taking periods
and with magnetic field pointing downwards. The unbinned maximum likelihood fit results are overlaid.}
\label{fig:unbinned:mass_KK}
\end{figure}
%%%%%%%%%%%%%%%%%%%%%%%%%%%%%%%%%%%%%

\begin{figure}[tbh]
\centering 
\includegraphics[width=0.49\textwidth]{Fig11a} 
\includegraphics[width=0.49\textwidth]{Fig11b} 
\caption{Distributions of (left) $m(\pip\pim)$ and (right) $\Delta m$ for the 
the selected \decay{\Dstar}{\Dz}{\pip}, \decay{\Dz}{\pip\pim}   candidates  
in the second of the three 2012 data taking periods
and with magnetic field pointing downwards. The unbinned maximum likelihood fit results are overlaid.}
\label{fig:unbinned:mass_PiPi}
\end{figure}
%%%%%%%%%%%%%%%%%%%%%%%%%%%%%%%%%%%%%

%%%%%%%%%%%%%%%%%
\begin{figure}[tbh]
\centering
\includegraphics[width=0.6\textwidth]{Fig12} 
\caption{Distribution of decay time for the selected \decay{\Dz}{\Kp\Km} candidates in the second of the
three 2012 data taking periods with magnetic field pointing downwards.
The unbinned maximum likelihood fit results are overlaid.}
\label{fig:unbinned:time_KK}
\end{figure}
%%%%%%%%%%%%%%%%%%%%%%%%%%%%%%%%%%%%%%%

%%%%%%%%%%%%%%%%%%
\begin{figure}[tbh]
\centering 
\includegraphics[width=0.494\textwidth]{Fig13a} 
\includegraphics[width=0.494\textwidth]{Fig13b} 
\caption{Distributions of (left) decay time and (right) $\ln(\chisqip(\Dz))$ 
for the selected \decay{\Dz}{\pip\pim}  candidates in the second of
the three 2012 data taking periods with magnetic field pointing downwards.
The unbinned maximum likelihood fit results are overlaid. Gaussian kernels are used to smooth the combinatorial backgrounds.}
\label{fig:unbinned:time_PiPi}
\end{figure}
%%%%%%%%%%%%%%%%%%%%%%%%%%%%%%%%%%%%%

%%%%%%%%%%%%%%%%%
\begin{figure}[tbh]
\centering
\includegraphics[width=0.8\textwidth]{Fig14} 
\caption{Asymmetry between \Dz and \Dzb data overlaid by the total unbinned maximum likelihood fit and prompt signal fit component for the \Kp\Km final state. 
The data are from all 2012 subsets and the fit components are constructed from the individual fits to each subset. 
The residuals between data and fit are shown in units of the statistical standard deviation, labelled as pull.}
\label{fig:unbinned:asym_KK}
\end{figure}
%%%%%%%%%%%%%%%%%%%%%%%%%%%%%%%%%%%%%

%%%%%%%%%%%%%%%%%
\begin{figure}[tbh]
\centering
\includegraphics[width=0.8\textwidth]{Fig15} 
\caption{Asymmetry between \Dz and \Dzb data overlaid by the total unbinned maximum likelihood fit and prompt signal 
fit component for the \pip\pim final state. The data are from all 2012 subsets and the fit components are constructed from the individual fits to each subset. 
The residuals between data and fit are shown in units of the statistical standard deviation, labelled as pull.}
\label{fig:unbinned:asym_PiPi}
\end{figure}
%%%%%%%%%%%%%%%%%%%%%%%%%%%%%%%%%%%%%
